# Supplementary material for: AuxMix: Semi-Supervised Learning with Unconstrained Unlabeled Data
Source: arXiv:2206.06959 source file (2022-06-14)
Supplement: Supplementary file 1 [file supplementary.tex]

\section{Supplementary materials}
\label{sec:supplementary}

Supplementary goes here.
